# Supplementary material for: Einstein Fields: A Neural Perspective To Computational General Relativity
Source: arXiv:2507.11589 source file (2026-02-09)
Supplement: Supplementary file 1 [file jax_advantages.tex]

\section{Accelerating computational differential geometry using JAX}\label{app_sec_jax}
\texttt{JAX} is a powerful high-performance numerical computing framework that  that is built on top of \texttt{XLA} (accelerated linear algebra), offering seamless executions of python-based functions on CPUs, GPUs and TPUs with minimal code modifications. It is an easy-to-use toolkit and is based on a  stateless, functional programming paradigm with \texttt{NumPy}-like syntax~\cite{harris2020numpy}, offering accelerator-backed execution capabilities. Our differential geometry toolkit Einstein Fields, leverages the following computational advantages offered by JAX: 
\begin{itemize}
    \item \emph{Automatic-Differentiation}: functionalities such as forward, reverse, Jacobian-vector product (\texttt{JVP}), Hessian-vector product (\texttt{HVP}) etc.) are capable of differentiating through complex control flows and perform complicated chain-rules on nested composition of maps. Additionally, effortless computation of higher order jets: \emph{Taylor-mode AD} for higher-order tensor derivatives~\cite{bettencourt2019taylormode}. 

    \item \texttt{XLA} \emph{Compilation}: By leveraging the XLA compiler, significant performance gains, particularly for compute-intensive workloads involving PDE solvers, large tensors and tensor operations. This is achieved via Just-In-Time (JIT) compilation feature, wherein Python functions are compiled into optimized machine code for the target hardware. 

    \item \emph{Automatic vectorization and parallelization}: automatically batch functions over array without manual loops: \texttt{jax.vmap} and  large-scale parallel simulations by distribution across multiple devices (e.g., multiple GPUs or TPU cores): \texttt{jax.pmap}. 

    \item \emph{Autoregressive rollouts}: efficient autoregressive rollout features by scanning over sequences (without manual loops): \texttt{jax.lax.scan}, offering speedups in time-stepping PDEs and so on. 

    \item \emph{PDE solvers}: Advanced applications including (neural) implicit and explicit PDE solvers using frameworks such as \texttt{Diffrax}.  
\end{itemize}
