# Supplementary material for: Einstein Fields: A Neural Perspective To Computational General Relativity
Source: arXiv:2507.11589 source file (2026-02-09)
Supplement: Supplementary file 2 [file table_of_notations.tex]

\begin{table}[H]
\centering
\caption{Table of Notation}
\begin{tabular}{ll}
\toprule
\textbf{Symbol} & \textbf{Description} \\
\midrule
$\mathcal{M}$ & Arbitrary manifold \\ 
$\mathscr{M}$ & 4-dimensional spacetime manifold \\
$ x^\mu $ & Spacetime coordinates, $\mu = 0,1,2,3$ \\
$ x^i $ & Spatial coordinates, $i = 1,2,3$ \\
$ g_{\mu\nu} $ & Spacetime metric tensor \\
$ g^{\mu\nu} $ & Inverse spacetime metric \\
$ \eta_{\mu\nu} $ & Minkowski metric, signature $(-+++)$ \\
$ \partial_\mu $ & Partial derivative with respect to $x^\mu$ \\
$ \nabla_\mu $ & Covariant derivative associated with $g_{\mu\nu}$ \\
$ \Gamma^\rho_{\mu\nu} $ & Christoffel symbols (connection coefficients) \\
$ R^\rho_{\ \sigma\mu\nu} $ & Riemann curvature tensor \\
$ R_{\mu\nu} $ & Ricci tensor, $R_{\mu\nu} = R^\rho_{\ \mu\rho\nu}$ \\
$ R $ & Ricci scalar, $R = g^{\mu\nu} R_{\mu\nu}$ \\
$ G_{\mu\nu} $ & Einstein tensor, $G_{\mu\nu} = R_{\mu\nu} - \frac{1}{2} R g_{\mu\nu}$ \\
$ T_{\mu\nu} $ & Energy-momentum (stress-energy) tensor \\
$ \Box = \nabla^\mu \nabla_\mu $ & D'Alembertian operator \\
$ \mathcal{L}_X $ & Lie derivative with respect to vector field $X$ \\
$ \epsilon_{\mu\nu\rho\sigma} $ & Levi-Civita tensor density (volume form) \\
$ \Sigma $ & Spacelike hypersurface \\
$ h_{ij} $ & Induced 3-metric on hypersurface $\Sigma$ \\
$ K_{ij} $ & Extrinsic curvature of $\Sigma$ \\
$ n^\mu $ & Unit normal vector to hypersurface $\Sigma$ \\
$ \delta^\mu_\nu $ & Kronecker delta \\
$ \mathcal{M} $ & Spacetime manifold \\
$ \mathcal{R} $, $ \mathcal{L} $ & Curvature scalar / Lagrangian density \\
$ c, G, \hbar $ & Speed of light, Newton’s constant, reduced Planck constant \\
\bottomrule
\end{tabular}
\label{tab:notation}
\end{table}
